# Supplementary material for: Adaptive Reward-Free Exploration
Source: arXiv:2006.06294 source file (2020-10-07)
Supplement: Supplementary file 1 [file appendix_H3.tex]

\section{Alternative algorithm for RF}

\begin{lemma}\label{lem:Bernstein_via_kl}
For $p,q\in\Sigma_S$ where we recall that we denote by $\Sigma_S$ the probability simplex of dimension $S-1$, for all $\alpha> 0 $, for all function $f$ defined on $\cS$ with $0\leq f(s) \leq B$ for all $s\in\cS$, if $\KL(p,q)\leq \alpha$ then
\begin{align*}
	 q f &\leq p f + \sqrt{2\Var_{q}(f)\alpha}+\frac{\alpha B}{3}\\
	 q f &\geq p f -\sqrt{2\Var_{q}(f)\alpha}-\frac{\alpha B}{3}\,.
\end{align*}
% \begin{align*}
% \up f &= \max_{p'\in\Sigma_S: \KL(p',p) < \alpha} q f \leq  p f + \sqrt{2\Var_{\up}(f)\alpha}+\frac{\alpha B}{3}\\
% \lp f &= \min_{p'\in\Sigma_S: \KL(p',p) < \alpha} q f \geq  p f - \sqrt{2\Var_{\lp}(f)\alpha}-\frac{\alpha B}{3}\,,
% \end{align*}
where we denote the expectation operator $pf = \EE_{s\sim p} f(s)$ and the variance operator
$\Var_p(f) = \EE_{s\sim p} \big(f(s)-\EE_{s'\sim p}f(s')\big)^2 = p(f-pf)^2$.
\end{lemma}
\begin{proof}
We only prove the fisrt inequality the proof of the second one is very similar. We assume that $q f > p f$ otherwise the inequality is trivially true and by homogeneity that for all $s\in\cS$, $0 \leq f(s) \leq 1$. Thanks to the variational formula for the Kullback-Leibler divergence we have
\begin{align*}
	\KL(p,q) &= \sup_{g \in \R^S} p g - \log(q e^{g})\\
	&\geq \sup_{\lambda\geq 0} \lambda(q f-pf) - \log(q e^{\lambda(q f -f)})\,,
\end{align*}
where we choose $g= q f -f$. Using that $\lambda \to (e^\lambda -\lambda -1)/\lambda$ is non-increasing and that $q f(s) -f(s) \leq 1$ one obtains
\[
e^{\lambda \big(q f -f(s)\big)} - \lambda\big( q f -f(s) \big) - 1 \leq \big(q f - f(s)\big)^2 (e^\lambda -\lambda-1)\,.
\]
Then by taking the expectation with respect to $q$ of the previous inequality, using $\log(1+x)\leq x$ and denoting the function $\phi(\lambda)= e^\lambda -\lambda -1$ we get
\begin{align*}
	\log(q e^{\lambda(q f-f)}) \leq \log\big(1+  \Var_{q}(f) \phi(\lambda)\big)\leq  \Var_{q}(f) \phi(\lambda)\,.
\end{align*}
Now using the previous inequality in the variational formula above with the fact that the convex conjugate of $\phi$ is for $u\geq 0$, $\sup_{\lambda\geq 0}\lambda u -\phi(\lambda) =: h(u) \geq u^2/\big(2(1+u/3)\big)$, yields
\begin{align*}
	\KL(p,q) &= \sup_{\lambda\geq 0} \lambda(q f-pf) -  \Var_{q}(f) \phi(\lambda)\\
	&\geq  \Var_{q}(f) h\left( \frac{q f-pf}{ \Var_{q}(f)}  \right)\\
	&\geq \frac{(q f-pf)^2}{2\Big(\Var_{q}(f)+(q f-pf)/3\Big)}\,.
\end{align*}
Since by definition $\KL(p,q) \leq \alpha$, we get
\[
2\alpha\Big(\Var_{q}(f)+(q f-pf)/3\Big)- (q f-pf)^2\geq 0\,,
\]
which allows us to conclude by finding the roots of this polynomial.
\end{proof}

\begin{lemma}
	\label{lem:switch_variance}
	For $p,q\in\Sigma_S$, for $f,g$ two functions defined on $\cS$ such that $0\leq g(s),f(s) \leq B$ for all $s\in\cS$,
	\begin{align*}
 \Var_p(f) &\leq 2 \Var_p(g) +2 B p|f-g|\\
 \Var_q(f) &\leq \Var_p(f) +3\|p-q\|_1 B^2\,,
\end{align*}
where we denote the absolute function $|f|(s)= |f(s)|$ for all $s\in\cS$.
\end{lemma}
\begin{proof}
First note that
\[
\Var_p(f-g) = p(f-g+ g-p g + p g- p f)^2 \leq 2 p(f-g - p f + p g)^2 +2 p(g-p g)^2 = 2\Var_p(f-g)+2\Var_p(g)\,.
\]
We can then conclude the poof of the first inequality with
\[
\Var_p(f-g) \leq p(f-g)^2 \leq B p|f-g|\,,
\]
where we used that for all $s\in\cS$, $0\leq f(s)-g(s) \leq B$. For the second inequality, thanks to the Holder inequality,
\begin{align*}
	\Var_q(f) &= pf^2 - (pf)^2 +(q-p)f^2 + (pf)^2 -(qf)^2 \\
	&\leq \Var_p(f) +\|p-q\|_1 B^2 +\|p-q\|_1 2B^2\\
	&\leq \Var_p(f) +3 B^2 \|p-q\|_1\,.
\end{align*}
\end{proof}

\begin{lemma}
	\label{lem:sum_1_over_n}
	 For $T\in\N^*$ and $(u_t)_{t\in\N^*}$ a sequence such that $u_t\in[0,1]$, for $U_t = \sum_{l=1}^t u_t$,
	\[
		\sum_{t=0}^T \frac{u_{t+1}}{U_t\vee 1} \leq 4\log(U_{T+1}+1)\,.
	\]
\end{lemma}
\begin{proof}
	We have
	\begin{align*}
		\sum_{t=0}^T \frac{u_{t+1}}{U_t\vee 1} &\leq 4 \sum_{t=0}^T \frac{u_{t+1} }{2U_t + 2} \\
		&\leq  4\sum_{t=0}^T \frac{U_{t+1}-U_{t}}{U_{t+1} + 1}\\
		&\leq 4\sum_{t=0}^T \int_{U_t}^{U_{t+1}} \frac{1}{x+1} \mathrm{d}x\\
		& = 4\log(U_{T+1}+1)\,.
	\end{align*}
\end{proof}

We now propose a more sophisticated sample complexity analysis, inspired by some tricks proposed by \citep{Azar17UCBVI}, which permits to obtain a bound that depends on the horizon in $H^3$, instead of $H^4$,for non-stationary transitions, when $\gamma = 1$.

\begin{theorem}\label{thm:sc_BPI_2} For general non-stationary transitions, for $0 < \epsilon \leq 1$, $\gamma=1$, the sample complexity of \OurAlgorithmBPI{} with the same threshold as in Theorem~\ref{thm:sc_BPI}, satisfies, with probability $1-\delta$,
\[
\tau \leq 4000 e \log(C_1) \left( \log(C_1)\log\left(\frac{2SAH}{\delta}\right)+2S\log(C_1) \right) \frac{H^3SA}{\epsilon^2}
\]
where
\[
C_1 = \frac{ 50000^4 H^{12}S^8A^4 \log\left(\frac{2SAH}{\delta}\right)^4 }{\epsilon^4}\,.
\]
In particular,
\[
\tau \leq \widetilde{O}\left( \frac{H^3SA}{\epsilon^2}\log\left(\frac{1}{\delta}\right)  \right)\,,\qquad \tau \leq \widetilde{O}\left( \frac{H^3S^2A}{\epsilon^2} \right)
\]
where $\widetilde{O}$ hides poly-log terms in $H,S,A,1/\epsilon,\log(1/\delta)$, in the first inequality and  poly-log terms in $H,S,A,1/\epsilon,1/\delta$, in the second inequality.
\end{theorem}

\begin{proof}
  The first part of the theorem is a direct consequence of the correctness of the confidence bounds. Indeed on the event $\cE$ if the algorithm stops at time $\tau$, then we know
 \begin{align*}
   V^{\lpi^\tau}_1(s_1) \geq \lV_1^{\tau,\lpi^\tau}(s_1) = \lV_1^\tau(s_1) \geq \uV_1^\tau(s_1) - \epsilon \geq \Vstar_1(s_1) - \epsilon\,.
 \end{align*}
 The fact that the event $\cE$ holds with probability at least $1-\delta$ allows us to conclude that \OurAlgorithmBPI is $(\varepsilon,\delta)$-correct.

 The proof of upper bounds on the complexity is very close to a classical regret proof. Fix
 some $T<\tau$. Then we know that for all $t\leq T$ it holds
 \[
\epsilon \leq  \uV_1^t(s_1)-\lV_1^t(s_1) \leq \uV_1^t(s_1)-\lV_1^{t,\upi^t}(s_1)\,.
 \]
We consider for the rest of the proof that the event $\cF$ holds. Note that this event holds with probability at least $1-\delta$. For a state action $(s,a)$ we have
\begin{align}
  \label{eq:decomposition_Q_BPI}
  \uQ_h^t(s,a)-\lQ^{t,\upi^t}_h(s,a) &= (\up_h^t-p_h) \uV_{h+1}^t(s,a) + (p_h-\lp_h^{t,\upi}) \lV_{h+1}^{t,\upi^t}(s,a) + p_h(\uV_{h+1}^t-\lV^{t,\upi^t}_{h+1})(s,a)\,.
\end{align}
We will upper-bound the first two terms of the left hand side separately. We first assume that $n_h^t(s,a)>0$ and decompose the first term as
\[
 (\up_h^t-p_h) \uV_{h+1}^t(s,a) = (\up_h^t-\hp_h^t) \uV_{h+1}^t(s,a) + (\hp_h^t-p_h) \uV_{h+1}^t(s,a)\,.
\]
We will use Lemma~\ref{lem:Bernstein_via_kl} to degrade the $ \KL$-confidence bounds to Bernstein type bounds. Thanks to Lemma~\ref{lem:Bernstein_via_kl} and the fact that we are on the event $\cE$, we can upper bound the first term in the above decomposition,
\begin{align*}
  (\up_h^t-\hp_h^t) \uV_{h+1}^t(s,a) \leq \sqrt{2\Var_{\up_h^t}(\uV_{h+1}^t)(s,a) \frac{\beta(n_h^t(s,a),\delta)}{n_h^t(s,a)}}+3 H\frac{ \beta(n_h^t(s,a),\delta)}{n_h^t(s,a)}\,,
\end{align*}
where we denote the variance operator $\Var_{p_h}(f)(s,a) = \EE_{s'\sim p_h(\cdot|s,a)}\big(f(s')-p_h f(s,a)\big)^2$. We will now relate the variance of the upper bound on the optimal value function under $\up_h$ to the variance of the optimal value function under $p_h$. Thanks to Lemma~\ref{lem:switch_variance} we obtain
\begin{align*}
  \Var_{\up_h^t}(\uV_{h+1}^t)(s,a) &\leq \Var_{p_h}(\uV_{h+1}^t)(s,a) + 3 H^2 \|\up_h^t(s,a) - p_h(s,a)\|_1\\
  &\leq \Var_{p_h}(\uV_{h+1}^t)(s,a) + 6 H^2 \frac{\beta(n_h^t(s,a),\delta)}{n_h^t(s,a)}\,,
\end{align*}
where we used the fact that $\uV_{h+1}^t \leq H$ and the Pinsker inequality. Using again the Lemma~\ref{lem:switch_variance} with $\uV_{h+1}^t \geq V^{\upi^{t}}_{h+1}$ yields
\[
\Var_{p_h}(\uV_{h+1}^t)(s,a) \leq 2\Var_{p_h}(V^{\upi^{t}}_{h+1})(s,a) + 2 H p_h(\uV_{h+1}^t-V^{\upi^{t}}_{h+1})(s,a)\,.
\]
Putting everything together and using successively $\sqrt{x+y}\leq\sqrt{x}+\sqrt{y}$ and $\sqrt{xy}\leq x+y$ one obtains
\begin{align*}
  (\up_h^t-\hp_h^t) \uV_{h+1}^t(s,a) &\leq \sqrt{4\Var_{p_h}(V^{\upi^{t}}_{h+1})(s,a) \frac{\beta(n_h^t(s,a),\delta)}{n_h^t(s,a)}}+ \sqrt{12} H \frac{\beta(n_h^t(s,a),\delta)}{n_h^t(s,a)} \\
  &\qquad+\sqrt{ \frac{1}{2 H} p_h(\uV_{h+1}^t-V^{\upi^{t}}_{h+1})(s,a)\frac{8 H^2 \beta(n_h^t(s,a),\delta)}{n_h^t(s,a)}} +3 H\frac{\beta(n_h^t(s,a),\delta)}{n_h^t(s,a)}\\
  &\leq 2\sqrt{\Var_{p_h}(V^{\upi^{t}}_{h+1})(s,a) \frac{\beta(n_h^t(s,a),\delta)}{n_h^t(s,a)}} +
   \frac{1}{2 H} p_h(\uV_{h+1}^t-V^{\upi^{t}}_{h+1})(s,a)\\
   &\qquad\qquad + 15 H^2\frac{ \beta(n_h^t(s,a),\delta)}{n_h^t(s,a)}\,,
\end{align*}
where we used the fact that $\sigma_H >1$. Similarly using Lemma~\ref{lem:Bernstein_via_kl} and Lemma~\ref{lem:switch_variance} (only the first part this time since we already have the variance under the probability $p_h$),
\begin{align*}
  (\hp_h^t-p_h) \uV_{h+1}^t(s,a) &\leq \sqrt{2\Var_{p_h}(\uV_{h+1}^t)(s,a) \frac{\beta(n_h^t(s,a),\delta)}{n_h^t(s,a)}}+3 H\frac{ \beta(n_h^t(s,a),\delta)}{n_h^t(s,a)} \\
  &\leq 2\sqrt{\Var_{p_h}(V^{\upi^{t}}_{h+1})(s,a) \frac{\beta(n_h^t(s,a),\delta)}{n_h^t(s,a)}} +
   \frac{1}{2 H} p_h(\uV_{h+1}^t-V^{\upi^{t}}_{h+1})(s,a) \\
   &\qquad\qquad+ 15 H^2\frac{ \beta(n_h^t(s,a),\delta)}{n_h^t(s,a)}\,.
\end{align*}
Thus combining these two upper bounds we have
\[
(\up_h^t-p_h) \uV_{h+1}^t(s,a) \leq  4\sqrt{\Var_{p_h}(V^{\upi^{t}}_{h+1})(s,a) \frac{\beta(n_h^t(s,a),\delta)}{n_h^t(s,a)}} +
 \frac{1}{ H} p_h(\uV_{h+1}^t-V^{\upi^{t}}_{h+1})(s,a) + 30 H^2\frac{ \beta(n_h^t(s,a),\delta)}{n_h^t(s,a)}\,.
\]
We can proceed in a similar way to upper bound the second term of the right hand side of \eqref{eq:decomposition_Q_BPI} using the second inequality of Lemma~\ref{lem:Bernstein_via_kl} and Lemma~\ref{lem:switch_variance} with the fact that $\lV_{h+1}^{t,\upi^t} \leq V^{\upi^{t}}_{h+1}$,
\begin{align*}
  (p_h-\lp_h^{t,\upi}) \lV_{h+1}^{t,\upi^t}(s,a) &=   (p_h-\hp_h^{t}) \lV_{h+1}^{t,\upi^t}(s,a)+   (\hp_h^{t}-\lp_h^{t,\upi}) \lV_{h+1}^{t,\upi^t}(s,a)\\
  &\leq 4\sqrt{\Var_{p_h}(V^{\upi^{t}}_{h+1})(s,a) \frac{\beta(n_h^t(s,a),\delta)}{n_h^t(s,a)}} +
   \frac{1}{H} p_h(V^{\upi^{t}}_{h+1}-\lV_{h+1}^{t,\upi^t})(s,a)\\
   &\qquad\qquad+ 30 H^2\frac{ \beta(n_h^t(s,a),\delta)}{n_h^t(s,a)}\,.
\end{align*}
We thus obtain by summing the two previous inequality an upper bound on the difference of Q-value functions in  \eqref{eq:decomposition_Q_BPI},
\begin{align*}
\uQ_h^t(s,a)-\lQ^{t,\upi^t}_h(s,a) &\leq  8\sqrt{\Var_{p_h}(V^{\upi^{t}}_{h+1})(s,a) \frac{\beta(n_h^t(s,a),\delta)}{n_h^t(s,a)}} + 60 H^2\frac{ \beta(n_h^t(s,a),\delta)}{n_h^t(s,a)}\\
 &\qquad\qquad+\gamma \left(1+\frac{1}{H}\right) p_h(\uV_{h+1}^t-\lV_{h+1}^{t,\upi^t})(s,a)\,.
\end{align*}
Then, since  it holds $\uQ_h^t(s,a)-\lQ^{t,\upi^t}_h(s,a) \leq H \leq  H^2$ we have for all $n_h^t(s,a)\in\N$,
\begin{align*}
  \uQ_h^t(s,a)-\lQ^{t,\upi^t}_h(s,a) &\leq  8\sqrt{\Var_{p_h}(V^{\upi^{t}}_{h+1})(s,a) \left[\frac{\beta(n_h^t(s,a),\delta)}{n_h^t(s,a)}\wedge 1\right]} + 60 H^2\left[\frac{ \beta(n_h^t(s,a),\delta)}{n_h^t(s,a)}\wedge 1\right]\\
  &\qquad\qquad+\left(1+\frac{1}{H}\right) p_h(\uV_{h+1}^t-\lV_{h+1}^{t,\upi^t})(s,a)\,.
\end{align*}
Thus, using that $\upi^t = \pi^{t+1}$ and by definition that $\uV_h^{t}(s) = \pi_h^{t+1}\uQ_h^{t}(s)$ and $\lV_h^{t,\upi^t}(s) = \pi_h^{t+1}\uQ_h^{t,\upi^t}(s)$, we obtain a recursive formula for the difference of upper and lower bound on the value functions
\begin{align*}
\uV_h^t(s)-\lV_h^{t,\upi^t}(s) &\leq 8\sqrt{\Var_{p_h}(V^{\pi^{t+1}}_{h+1})(s,a) \left[\frac{\beta(n_h^t(s,a),\delta)}{n_h^t(s,a)}\wedge 1\right]} + 60 H^2\left[\frac{ \beta(n_h^t(s,a),\delta)}{n_h^t(s,a)}\wedge 1\right]\\
&\qquad\qquad+\left(1+\frac{1}{H}\right) p_h(\uV_{h+1}^t-\lV_{h+1}^{t,\upi^t})(s,a)\,.
\end{align*}
Denoting by $p_h^{t}(s,a)$  the probability of reaching state action $(s,a)$ at step $h$ under the policy $\pi^t$, we get by induction with the previous formula
\begin{align*}
\epsilon &\leq \uV_1^t(s)-\lV_1^{t,\upi^t}(s)\\
&\leq \sum_{h=1}^H\sum_{s,a} p_h^{t+1}(s,a) e\Bigg(8\sqrt{\Var_{p_h}(V^{\pi^{t+1}}_{h+1})(s,a) \left[\frac{\beta(n_h^t(s,a),\delta)}{n_h^t(s,a)}\wedge 1\right]} + 60 H^2\left[\frac{ \beta(n_h^t(s,a),\delta)}{n_h^t(s,a)}\wedge 1\right]\Bigg)\,,
\end{align*}
where we used that $(1+1/H)^H\leq e$. Thus, summing for all $0\leq t \leq T$, using Lemma~\ref{lem:cnt_pseudo} and that $\beta(\bar{n}_h^t(s,a),\delta)\leq \beta(T,\delta)$ for all $t\leq T$ then the Cauchy-Schwarz inequality, leads to
\begin{align*}
  (T+1)\epsilon &\leq  16e\sqrt{\beta(T,\delta)}\sum_{t=0}^T\sum_{h=1}^H\sum_{s,a} p_h^{t+1}(s,a) \sqrt{\Var_{p_h}(V^{\upi^{t}}_{h+1})(s,a) \frac{1}{\bn_h^t(s,a)\vee 1}}\\
  &\qquad\qquad + 240e\beta(T,\delta) H^2 \sum_{t=0}^T\sum_{h=1}^H\sum_{s,a} p_h^{t+1}(s,a)
   \frac{1}{\bn_h^t(s,a)\vee 1}\\
   &\leq 16e\sqrt{\beta(T,\delta)} \sqrt{\sum_{t=0}^T\sum_{h=1}^H\sum_{s,a} p_h^{t+1}(s,a) \Var_{p_h}(V^{\pi^{t+1}}_{h+1})(s,a)}\sqrt{\sum_{t=0}^T\sum_{h=1}^H\sum_{s,a} p_h^{t+1}(s,a)
    \frac{1}{\bn_h^t(s,a)\vee 1}} \\
    &\qquad\qquad + 240e\beta(T,\delta) H^2 \sum_{t=0}^T\sum_{h=1}^H\sum_{s,a} p_h^{t+1}(s,a)
     \frac{1}{\bn_h^t(s,a)\vee 1}\,.
\end{align*}

% \todoe{What is the Bellman equations for the variances? Is it given above or is it in some Azar paper?}

On one hand, using the Bellman-type recursive law of total variance, see \citep{zanette2019tighter}, we can upper bound the sum involving the variances in the inequality above
\begin{align*}
\sum_{t=0}^T\sum_{h=1}^H\sum_{s,a} p_h^{t+1}(s,a) \Var_{p_h}(V^{\pi^{t+1}}_{h+1})(s,a) &\leq \sum_{t=0}^T \EE_{\pi^{t+1}}\!\!\left[ \left(\sum_{h=1}^H r_h(s_h,a_h) -V_1^{\pi^{t+1}}(s_1)\right)^2\right] \\
&\leq H^2 (T+1)\,.
\end{align*}
On the other hand, thanks to Lemma~\ref{lem:sum_1_over_n}, we get
\begin{align*}
\sum_{t=0}^T\sum_{h=1}^H\sum_{s,a} p_h^{t+1}(s,a)
 \frac{1}{\bn_h^t(s,a)\vee 1} &= \sum_{h=1}^H\sum_{s,a} \sum_{t=0}^T \frac{\bn_h^{t+1}(s,a) -\bn_h^t(s,a)}{\bn_h^t(s,a)\vee 1}\\
 &\leq 4H SA\log(T+1)\,.
\end{align*}
Combining these two inequalities with the previous one we obtain
\begin{align*}
  (T+1)\epsilon &\leq  32e\sqrt{\beta(T,\delta) H^3 SA (T+1)\log(T+1)} + 960 e \beta(T,\delta) H^3 SA \log(T+1)\,.
\end{align*}
We assume now that $\tau>0$ otherwise the result is trivially true. Since the inequality above is true for all $T<\tau$, using that
\[
\beta(T,\delta) \leq \log\!\!\left(\frac{2SAH}{\delta}\right)+2S\log(\tau)\,,
\]
it holds
\begin{align}
  \epsilon \tau  &\leq  32e\sqrt{\left(\log\!\!\left(\frac{2SAH}{\delta}\right)+2S\log(\tau)\right) H^3 SA \tau\log(\tau)} \nonumber\\
  &\qquad\qquad+ 960 e \left(\log\!\!\left(\frac{2SAH}{\delta}\right)+2S\log(\tau)\right)  H^3 SA \log(\tau)\label{eq:to_inverse_BPI}\,.
\end{align}
The end of the proof is a bit technical since we need to inverse~\eqref{eq:to_inverse_BPI} to obtain a bound on $\tau$. Using that for all $\alpha\in(0,1]$, for $x\geq 1$ it holds $\log(x)\leq x^\alpha /\alpha$, one can upper-bound
\begin{align*}
  \left(\log\!\!\left(\frac{2SAH}{\delta}\right)+2S\log(\tau)\right) H^3 SA \tau\log(\tau)
  &\leq 2H^3SA  \log\!\!\left(\frac{2SAH}{\delta}\right) \tau^{3/2}+32H^3S^2A\tau^{3/2}\\
  &\leq 34 H^3S^2A \log\!\!\left(\frac{2SAH}{\delta}\right)\tau^{3/2}.
\end{align*}
Thus we have
\begin{align*}
32e\sqrt{\left(\log\left(\frac{2SAH}{\delta}\right)+2S\log(\tau)\right) H^3 SA \tau\log(\tau)}&\leq 508 \sqrt{ H^3S^2A \log\left(\frac{2SAH}{\delta}\right)\tau^{3/2}}\\
&\leq  508  H^3S^2A \log\left(\frac{2SAH}{\delta}\right) \tau^{3/4}\,.
\end{align*}
Similarly we can upper-bound the second in the right hand term of~\eqref{eq:to_inverse_BPI}
\begin{align*}
  \left(\log\left(\frac{2SAH}{\delta}\right)+2S\log(\tau)\right)  H^3 SA \log(\tau)&\leq
  2H^3SA \log\left(\frac{2SAH}{\delta}\right) \tau^{3/4}+15H^3S^2A\tau^{3/4}\\
  &\leq 17 H^3S^2A \log\left(\frac{2SAH}{\delta}\right)\tau^{3/4}\,.
\end{align*}
Plugging this two inequalities in~\eqref{eq:to_inverse_BPI} leads to
\[
\epsilon \tau \leq 50000 H^3SA \log\left(\frac{2SAH}{\delta}\right) \tau^{3/4}\,,
\]
which gives the raw upper-bound on $\tau$,
\begin{equation}
\tau \leq C_1 := \frac{ 50000^4 H^{12}S^8A^4 \log\left(\frac{2SAH}{\delta}\right)^4 }{\epsilon^4}\,.\label{eq:def_C1_BPI}
\end{equation}
Plugging back this bound in~\eqref{eq:to_inverse_BPI} leads to
\begin{align*}
  \epsilon \tau &\leq  32e\sqrt{\log(C_1)\left(\log\left(\frac{2SAH}{\delta}\right)+2S\log(C_1)\right) H^3 SA \tau} \\
  &+ 960 e \log(C_1)\left(\log(C_1)\log\left(\frac{2SAH}{\delta}\right)+2S\log(C_1)\right)  H^3 SA\\
  &\leq 2\sqrt{C_2 \tau} +C_2\,,
\end{align*}
where we denote
\[
C_2 :=   960 e \log(C_1)\left(\log(C_1)\log\left(\frac{2SAH}{\delta}\right)+2S\log(C_1)\right)  H^3 SA\,.
\]
Finding the roots of the polynomial $\epsilon x^2 - 2\sqrt{C_2} x - C_2$ and using the fact that $\epsilon\leq 1$, yields the upper bound on the stopping time,
\begin{align*}
  \tau &\leq \left(\frac{\sqrt{C_2}+ \sqrt{(1-\epsilon)C_2}}{\epsilon}\right)^2\\
  &\leq \frac{4C_2}{\epsilon^2}\\
  &\leq 4000 e \log(C_1) \left( \log(C_1)\log\left(\frac{2SAH}{\delta}\right)+2S\log(C_1) \right) \frac{H^3SA}{\epsilon^2}\,.
\end{align*}
Recalling the definition of $C_1$ in~\eqref{eq:def_C1_BPI} we can conclude that
\[
\tau \leq \widetilde{O}\left( \frac{H^3SA}{\epsilon^2}\log\left(\frac{1}{\delta}\right)  \right)\,,\qquad \tau \leq \widetilde{O}\left( \frac{H^3S^2A}{\epsilon^2} \right)
\]
where $\widetilde{O}$ hides poly-log terms in $H,S,A,1/\epsilon,\log(1/\delta)$, in the first inequality and  poly-log terms in $H,S,A,1/\epsilon,1/\delta$, in the second inequality.
% Letting $T_0$ be the smallest $T$ such that \[960 e \beta(T,\delta) H^3 SA \log(T+1) < e\sqrt{\beta(T,\delta) H^3 SA (T+1)\log(T+1)},\]
% for all $T_0 < T < \tau$, one has
% \begin{align*}
%   (T+1)\epsilon &\leq  (33e)^2H^3 SA\beta(T+1,\delta)\log(T+1)\,.
% \end{align*}
% The end of the proof is a bit technical, since we nee

\end{proof}

We assume that the event $\cF$ holds, and fix a policy $\pi$. Thanks to Lemma~\ref{lem:Bernstein_via_kl} we know that for a state action $(s,a)$ if $n_h^t(s,a)>0$,
\begin{align}
  \hQ_h^{t,\pi}(s,a)-Q_h^\pi(s,a) &= (\hp_h^{t}-p_h)V_{h+1}^{\pi}(s,a)+\hpi_h^t(\hV^{t,\pi}_{h+1}-V_{h+1}^pi)(s,a)\nonumber\\
  &\leq \sqrt{2 \Var_{p_h}(V_{h+1}^\pi) \frac{\beta(n_h^t(s,a),\delta)}{n_h^t(s,a)}}+H\frac{\beta(n_h^t(s,a),\delta)}{3n_h^t(s,a)}+\hp_h^t(\hV_{h+1}^{t,\pi}-V_{h+1}^\pi)(s,a)\label{eq:initial_bound_H3}\,.
\end{align}
But, thanks to Lemma~\ref{lem:switch_variance} with the fact that $0\leq V_{h+1}^\pi \leq H$ and to the Pinsker inequality  we get
\begin{align*}
  \Var_{p_h}(V_{h+1}^\pi)(s,a) &\leq \Var_{\hp_h^t}(V_{h+1}^\pi)(s,a) +3 H^2\|\hp_h^t(s,a)-p_h(s,a)\|_1\\
  &\leq \Var_{\hp_h^t}(V_{h+1}^\pi)(s,a) +3H^2\frac{\beta(n_h^t(s,a),\delta)}{n_h^t(s,a)}\,.
\end{align*}
Using again the Lemma~\ref{lem:switch_variance} we can replace the value function by its estimate
\[
\Var_{\hp_h^t}(V_{h+1}^\pi)(s,a)  \leq 2 \Var_{\hp_h^t}(\hV_{h+1}^{t,\pi})(s,a)+2H\hp_{h}^t|V_{h+1}^\pi -\hV_{h+1}^{t,\pi}|(s,a)\,.
\]
Combining these two inequalities one obtains
\begin{align*}
  \sqrt{2 \Var_{p_h}(V_{h+1}^\pi) \frac{\beta(n_h^t(s,a),\delta)}{n_h^t(s,a)}} &\leq 2\sqrt{ \Var_{\hp_h^t}(\hV_{h+1}^{t,\pi}) \frac{\beta(n_h^t(s,a),\delta)}{n_h^t(s,a)}}+\sqrt{6}H \frac{\beta(n_h^t(s,a),\delta)}{n_h^t(s,a)}\\
  &\qquad\qquad+ \sqrt{\frac{1}{H} \hp_h^t|V_{h+1}^\pi -\hV_{h+1}^{t,\pi}|(s,a) 4H^2\frac{\beta(n_h^t(s,a),\delta)}{n_h^t(s,a)}}\\
  &\leq 2\sqrt{ \Var_{\hp_h^t}(\hV_{h+1}^{t,\pi}) \frac{\beta(n_h^t(s,a),\delta)}{n_h^t(s,a)}} + (\sqrt{6}H+4H^2)\frac{\beta(n_h^t(s,a),\delta)}{n_h^t(s,a)}\\
  &\qquad\qquad+ \frac{1}{H}\hp_{h}^t|V_{h+1}^\pi -\hV_{h+1}^{t,\pi}|(s,a)\,.
\end{align*}
Injecting this inequality in the initial bound~\eqref{eq:initial_bound_H3} on the difference of Q-values and taking the absolute value yields
\begin{align*}
  |\hQ_h^{t,\pi}(s,a)-Q_h^\pi(s,a)| &\leq 2\sqrt{ \frac{\Var_{\hp_h^t}(\hV_{h+1}^{t,\pi})(s,a)}{H^2} \frac{H^2\beta(n_h^t(s,a),\delta)}{n_h^t(s,a)}} + 7H^2\frac{\beta(n_h^t(s,a),\delta)}{n_h^t(s,a)}\\
  &\qquad\qquad+\left(1+\frac{1}{H}\right)\hp_h^t |V_{h+1}^\pi -\hV_{h+1}^{t,\pi}|(s,a)\\
  &\leq  2\sqrt{ \frac{\Var_{\hp_h^t}(\hV_{h+1}^{t,\pi})(s,a)}{H^2} \left(\frac{H^2\beta(n_h^t(s,a),\delta)}{n_h^t(s,a)}\wedge 1\right)} +9H^2\frac{\beta(n_h^t(s,a),\delta)}{n_h^t(s,a)}\\
  &\qquad\qquad+\left(1+\frac{1}{H}\right)\hp_h^t |V_{h+1}^\pi -\hV_{h+1}^{t,\pi}|(s,a)
\end{align*}
where in the last inequality we used that if $H^2\beta(n_h^t(s,a),\delta)/n_h^t(s,a)\geq 1$ then
\[
2\sqrt{ \frac{\Var_{\hp_h^t}(\hV_{h+1}^{t,\pi})(s,a)}{H^2} \frac{H^2\beta(n_h^t(s,a),\delta)}{n_h^t(s,a)}} \leq 2\sqrt{\frac{H^2\beta(n_h^t(s,a),\delta)}{n_h^t(s,a)}} \leq 2 \frac{H^2\beta(n_h^t(s,a),\delta)}{n_h^t(s,a)}\,.
\]
We thus obtain the following bound on the error of estimation of the Q-value function at state action $(s,a)$ if $n_h^t(s,a)>0$,
\begin{align*}
  \he_h^{t,\pi}(s,a) &\leq 2\sqrt{ \frac{\Var_{\hp_h^t}(\hV_{h+1}^{t,\pi})(s,a)}{H^2} \left(\frac{H^2\beta(n_h^t(s,a),\delta)}{n_h^t(s,a)}\wedge 1\right)} +9H^2\frac{\beta(n_h^t(s,a),\delta)}{n_h^t(s,a)}\\
  &\qquad\qquad+\left(1+\frac{1}{H}\right)\hp_h^t \pi_{h+1} \he_{h+1}^{t,\pi}(s,a)
\end{align*}
where we recall $\pi_{h} f (s')= f(s',\pi_h(s')$. Thus, defining recursively the functions, $Z_{H+1}^{t,\pi}(s,a)=0$ and
\begin{align*}
  Z_h^{t,\pi}(s,a) &=\min\!\!\Bigg(H, 2\sqrt{ \frac{\Var_{\hp_h^t}(\hV_{h+1}^{t,\pi})(s,a)}{H^2} \left(\frac{H^2\beta(n_h^t(s,a),\delta)}{n_h^t(s,a)}\wedge 1\right)} +9H^2\frac{\beta(n_h^t(s,a),\delta)}{n_h^t(s,a)}\\
 &\qquad\qquad+\left(1+\frac{1}{H}\right)\hp_h^t \pi_{h+1} Z_{h+1}^{t,\pi}(s,a)\Bigg)
\end{align*}
and noting that $  \he_h^{t,\pi}(s,a) \leq H$ we can prove by induction that for all $h,s,a$
\begin{equation}
  \label{eq:he_lower_Z_H3}
\he_h^{t,\pi}\leq Z_h^{t,\pi}(s,a)\,.
\end{equation}
We now define recursively two other quantities for all $(s,a)$, by $Y_{H+1}^{t,\pi}(s,a)=W_{H+1}^{t,\pi}(s,a)=0$ and
\begin{align*}
  Y_h^{t,\pi}(s,a) &= 2\sqrt{ \frac{\Var_{\hp_h^t}(\hV_{h+1}^{t,\pi})(s,a)}{H^2} \left(\frac{H^2\beta(n_h^t(s,a),\delta)}{n_h^t(s,a)}\wedge 1\right)} + \left(1+\frac{1}{H}\right)\hp_h^t \pi_{h+1} Y_{h+1}^{t,\pi}(s,a)\\
  W_h^{t}(s,a) &=\min\!\!\left(H, 9H^2 \frac{\beta(n_h^t(s,a),\delta)}{n_h^t(s,a)} +\left(1+\frac{1}{H}\right)\hp_h^t \pi_{h+1} W_{h+1}^{t,\pi}(s,a) \right)
\end{align*}
We can prove by induction that for all $h,s,a$
\[
Z_h^{t,\pi}(s,a) \leq Y_h^{t,\pi}(s,a)+W_h^{t}(s,a)\,.
\]
Inded the case $h=H+1$ is trivially true and if we assume the inequality true at step $h+1$ then using that $\min(x,y+z)\leq \min(x,y)+\min(x,z)$ for $x,y,z\geq 0$,
\begin{align*}
  Z_h^{t,\pi}(s,a) &\leq  \min\Bigg(H, 2\sqrt{ \frac{\Var_{\hp_h^t}(\hV_{h+1}^{t,\pi})(s,a)}{H^2} \left(\frac{H^2\beta(n_h^t(s,a),\delta)}{n_h^t(s,a)}\wedge 1\right)} +9H^2\frac{\beta(n_h^t(s,a),\delta)}{n_h^t(s,a)}\\
 &\qquad\qquad+\left(1+\frac{1}{H}\right)\hp_h^t \pi_{h+1} Y_{h+1}^{t,\pi}(s,a)+\left(1+\frac{1}{H}\right)\hp_h^t \pi_{h+1} W_{h+1}^{t,\pi}(s,a)\Bigg)\\
 &\leq  Y_h^{t,\pi}(s,a)+W_h^{t}(s,a).
\end{align*}
Then using~\eqref{eq:he_lower_Z_H3} we have
\begin{equation}\label{eq:he_lower_YpW_H3}
\pi_1 \he_1^{t,\pi}(s_1) \leq \pi_1 Y_1^{t,\pi}(s_1)+\pi_1 W_1^{t,\pi}(s_1)\,.
\end{equation}
Now we will upper bound the term with $Y_h^{t,\pi}$ to make disappear the dependency in the empirical variances of the the value function of the policy $\pi$.
We denote by $\hpi_h^{t,\pi}(s,a)$ the probability to reach the sate-action $(s,a)$ at step $h$ under the policy $\pi$ with the empirical transitions at time $t$. Using successively the definition of the $Y_h^{t,\pi}$, the Cauchy-Schwarz inequality, and the Bellman-type law of total variation (see~\citep{zanette2019tighter}) we get
\begin{align*}
  \pi Y_1^{t,\pi}(s_1) &= 2\sum_{s,a}\sum_{h=1}^H \hp_h^{t,\pi}(s,a) \left(1+\frac{1}{H}\right)^{h-1}  2\sqrt{ \frac{\Var_{\hp_h^t}(\hV_{h+1}^{t,\pi})(s,a)}{H^2} \left(\frac{H^2\beta(n_h^t(s,a),\delta)}{n_h^t(s,a)}\wedge 1\right)}\\
  &\leq 2e \sqrt{\sum_{s,a}\sum_{h=1}^H \hp_h^{t,\pi}(s,a)\frac{ \Var_{\hp_h^t}(\hV_{h+1}^{t,\pi})(s,a)}{H^2}}\sqrt{\sum_{s,a}\sum_{h=1}^H \hp_h^{t,\pi}(s,a) \left(\frac{H^2\beta(n_h^t(s,a),\delta)}{n_h^t(s,a)}\wedge 1\right)}\\
  &\leq 2e \sqrt{\frac{1}{H^2}  \EE_{\pi, \hp_h^t}\!\!\left[ \left(\sum_{h=1}^H r_h(s_h,a_h) -\hV_1^{\pi}(s_1)\right)^2\right]  }\sqrt{\sum_{s,a}\sum_{h=1}^H \hp_h^{t,\pi}(s,a) \left(\frac{H^2\beta(n_h^t(s,a),\delta)}{n_h^t(s,a)}\wedge 1\right)}\\
  &\leq 2e\sqrt{\sum_{s,a}\sum_{h=1}^H \hp_h^{t,\pi}(s,a) \left(\frac{H^2\beta(n_h^t(s,a),\delta)}{n_h^t(s,a)}\wedge 1\right)}\,.
\end{align*}
Now we define recursively the quantity $\tW^{t,\pi}$ by: $\tW_{H+1}^{t,\pi}(s,a)=0$ and
\[
\tW_{h}^{t,\pi}(s,a) = \left(\frac{H^2\beta(n_h^t(s,a),\delta)}{n_h^t(s,a)}\wedge 1\right) + \hp_h^{t,\pi} \pi_{h+1} \tW_{h+1}^{t,\pi}(s,a)\,,
\]
such that by construction
\[
\sum_{s,a}\sum_{h=1}^H \hp_h^{t,\pi}(s,a) \left(\frac{H^2\beta(n_h^t(s,a),\delta)}{n_h^t(s,a)}\wedge 1\right) = \pi_1 \tW_1^{t,\pi}(s_1)\,.
\]
By induction we can prove that $\tW_h^{t,\pi}\leq W_h^{t,\pi}$. Indeed, the inequality is true for $h=H+1$ and if we assume it is true for step $h+1$ then using that by construction $\tW_{h}^{t,\pi}(s,a)\leq H$, for all $s,a$,
\begin{align*}
  \tW_{h}^{t,\pi}(s,a) &=\min\!\!\left(H, \left(\frac{H^2\beta(n_h^t(s,a),\delta)}{n_h^t(s,a)}\wedge 1\right) + \hp_h^{t,\pi} \pi_{h+1} \tW_{h+1}^{t,\pi}(s,a)\right)\\
  &\leq \min\!\!\left(H, \frac{H^2\beta(n_h^t(s,a),\delta)}{n_h^t(s,a)} + \hp_h^{t,\pi} \pi_{h+1} W_{h+1}^{t,\pi}(s,a)\right)\\
  &\leq W_{h}^{t,\pi}(s,a)\,.
\end{align*}
Thus we just proved that $ \pi_1 Y_1^{t,\pi}(s_1)\leq 2e \sqrt{\pi_1 W_1^{t,\pi}(s_1)}$ and going back to~\eqref{eq:he_lower_YpW_H3} we get
\begin{equation}
  \label{eq:he_lower_W_H3}
  \pi_1 \he_1^{t,\pi}(s_1) \leq  2e \sqrt{\pi_1 W_1^{t,\pi} (s_1)} + \pi_1 W_1^{t,\pi}(s_1)\,.
\end{equation}
Since $W_1^{t,\pi}$ control the error and does not depend on the rewards we can define a policy that acts greedily with respect to it. Precisely we introduce:
$W_{H+1}^{t}(s,a)=0$ for all $(s,a)$ and define recursively for all $h\in[H]$
\[
W_h^{t}(s,a) = \min\!\!\left(H, 9H^2 \frac{\beta(n_h^t(s,a),\delta)}{n_h^t(s,a)} +\left(1+\frac{1}{H}\right)\sum_{s'}\hp_h^t(s'|s,a) \max_{a'} W_{h+1}^{t}(s',a') \right)\,.
\]
 We thus introduce the algorithm \OurAlgorithmH:
\begin{itemize}
 \item \textbf{sampling rule}: the policy $\pi^{t+1}$ is the greedy policy with respect to $W_h^{t}$, that is
  \[\forall s \in \cS, \forall h \in [h], \ \ \pi^{t+1}_h(s) = \text{argmax}_a W_h^{t}(s,a).\]
 \item \textbf{stopping rule}: $\tau = \inf \left\{ t\in \N : 2e \sqrt{\pi_1^{t+1} W_1^{t,} (s_1)} + \pi_1^{t+1} W_1^{t}(s_1)  \leq \varepsilon/2 \right\}$.
\end{itemize}
Note that contrary to \OurAlgorithm that use bonus of the form $\sqrt{\beta(n_h^t(s,a),\delta)/n_h^t(s,a)}$ this algorithm just considers bonuses of the form $\beta(n_h^t(s,a),\delta)/n_h^t(s,a)$.
\begin{remark}
Note that on the event $\cE$ we have
\[
\KL\big(\hat{p}^t_h(\cdot | (s,a)), p_h(\cdot | (s,a))\big)\leq \tfrac{\beta(n_h^t(s,a),\delta)}{n_h^t(s,a)}\,.
\]
Thus ignoring the clipping and possibly infinite terms we have
\[
\pi_1 W_1^{t,\pi}(s_1) \gtrsim \sum_{h=1}^H \sum_{s,a} \hp_h^{t,\pi}(s,a) \KL\big(\hat{p}^t_h(s,a), p_h(s,a)\big) = \KL( \hp_H^{t,\pi}, \hp_H^\pi)\,,
\]
where we used the chain rule for the last inequality. Thus we can see \OurAlgorithmH as minimizing the Kullback-Leibler divergence between the state-action distribution in the empirical MDP and the one in the true MDP. And, from far, \OurAlgorithmH is somewhat an optimistic version of the MaxEnt algorithm proposed by~\citep{hazan2018provably}.
\end{remark}
